# Supplementary material for: Collisionless Transport Close to a Fermionic Quantum Critical Point in Dirac Materials
Source: arXiv:1801.03495 source file (2018-09-28)
Supplement: Supplementary file 1 [file Supplementary_GNYOC_2.pdf]

# Supplementary Materials: Collisionless Transport Close to a Fermionic Quantum Critical Point in Dirac Materials

Bitan Roy[1] and Vladimir Juričić[2]

[1]Max-Planck-Institut für Physik komplexer Systeme, Nöthnitzer Stra. 38, 01187 Dresden, Germany

[2]Nordita, KTH Royal Institute of Technology and Stockholm University, Roslagstullsbacken 23, 10691 Stockholm, Sweden

In the Supplementary Materials we present the details of the following analyses:

1. Computation of fermionic self-energy due to Yukawa interaction at finite temperature ($T$), and the additional correction to the optical conductivity (OC) at the superconducting Gross-Neveu-Yukawa (GNY) quantum critical point (QCP) due to gapless bosonic excitations of charge $2e$,

2. Computation of the thermal fermionic mass $[m_f(T)]$ in the critical regime of GNY QCP,

3. Derivation of the Drude conductivity for Dirac femrions.

## I. FERMIONIC SELF-ENERGY AT FINITE TEMPERATURE

To extract the scaling of optical conductivity (OC) at the GNY QCP at finite temperature we need the expression for the fermionic self-energy correction due to Yukawa coupling at finite-$T$ but only in the presence of external frequency. Formally the expression reads as

$$\Sigma(i\Omega) = g^2 \, N_b \, T \sum_{\omega_n} \int \frac{d^d\mathbf{q}}{(2\pi)^d} \, \frac{i\omega_n}{[\omega_n^2+q^2]\left[(\omega_n-\Omega)^2+q^2\right]} = ig^2 \, N_b \int \frac{d^d\mathbf{q}}{(2\pi)^d} \, F\left(q, i\Omega, T\right), \tag{1}$$

where

$$F\left(q, i\Omega, T\right) = -\frac{q}{\Omega\left(4q^2+\Omega^2\right)} \tanh\left(\frac{q}{2T}\right) + \sum_{\tau=\pm} \frac{q+i\tau\Omega}{4q\Omega(2q+i\tau\Omega)} \, \tanh\left(\frac{q+i\tau\Omega}{2T}\right). \tag{2}$$

Now we add and subtract the $T=0$ part of the self-energy to write the above expression compactly as

$$\Sigma(i\Omega) = ig^2 \, N_b \, \left\{ \int \frac{d^d\mathbf{q}}{(2\pi)^d} \left[F\left(q, i\Omega, T\right) - F\left(q, i\Omega, 0\right)\right] + \int \frac{d^d\mathbf{q}}{(2\pi)^d} F\left(q, i\Omega, 0\right) \right\}. \tag{3}$$

The fermionic wave-function renormalization $Z_\Psi$ can then be extracted from the following renormalization condition

$$i\Omega Z_\Psi(i\Omega) + \Sigma(i\Omega) = i\Omega. \tag{4}$$

From the above expression we can compactly write $Z_\Psi(i\Omega) = 1 + Z^{(1)}_\Psi(i\Omega) + Z^{(2)}_\Psi(i\Omega)$, where

$$Z^{(1)}_\Psi(i\Omega) = -ig^2 \, N_b \, \left\{ \frac{1}{i\Omega} \int \frac{d^d\mathbf{q}}{(2\pi)^d} \left[F\left(q, i\Omega, T\right) - F\left(q, i\Omega, 0\right)\right] \right\}, \quad Z^{(2)}_\Psi(i\Omega) = -ig^2 \, N_b \, \left\{ \frac{1}{i\Omega} \int \frac{d^d\mathbf{q}}{(2\pi)^d} F\left(q, i\Omega, 0\right) \right\}. \tag{5}$$

Notice that $Z^{(1)}_\Psi(i\Omega)$ is finite at $d=3$, while $Z^{(2)}_\Psi(i\Omega)$ exhibits a logarithmic divergence, which we capture by performing the momentum integral in dimension $d = 3-\epsilon$. We first present the computation of $Z^{(1)}_\Psi(i\Omega)$.

After rescaling the momentum variable as $q/\Omega \to q$ and subsequently performing analytical continuation as $i\Omega \to \omega + i\delta$ we arrive at $Z^{(1)}_\Psi(x) = -g^2 N_b f_1(x)/2$ in terms of dimensionless coupling constant $g^2\Omega^{-\epsilon}/(8\pi^2) \to g^2$, where $x = \omega/T$ and

$$f_1(x) = 2\int_0^\infty dq \, \frac{q}{4q^2-1} \, \left\{ 4q^2 \tanh\left(\frac{qx}{2}\right) - 2\frac{\cosh(qx) + \cosh(q) + (2q^2-1)\sinh(qx) + q\sinh(x)}{\cosh(qx)+\cosh(x)} \right\}, \tag{6}$$

while $f_1(x \to \infty) \approx 2.18486$ (obtained numerically). On the other hand, computation of $Z^{(2)}_\Psi(i\Omega)$ goes as follows

$$Z^{(1)}_\Psi(i\Omega) = -\frac{ig^2\, N_b}{2i\Omega} \int \frac{d^d\mathbf{q}}{(2\pi)^d} \frac{\Omega}{q\,(4q^2+\Omega^2)} = -g^2 \frac{S_d\, N_b}{2(2\pi)^d} \int_0^\infty dq\, \frac{q^{d-2}}{4q^2+\Omega^2} = g^2\, N_b\, \frac{2\pi^{1+d/2}\Omega^{-\epsilon}}{2^{d+1}\Gamma(d/2)(2\pi)^d} \sec\left(\frac{\pi d}{2}\right). \quad (7)$$

Now in dimension $d = 3-\epsilon$ and in terms of the dimensionless coupling constant $g^2\Omega^{-\epsilon}/(8\pi^2) \to g^2$ the above expression reads as

$$Z^{(1)}_\Psi(i\Omega) = -\frac{g^2}{2}\, N_b \left[\frac{1}{\epsilon} + \frac{2+\ln(4\pi)-\gamma_E}{2}\right] + \mathcal{O}(\epsilon) \equiv -\frac{g^2}{2}\, N_b \left[\frac{1}{\epsilon} + b\right] + \mathcal{O}(\epsilon), \quad (8)$$

where $b = [2+\ln(4\pi)-\gamma_E]/2 \approx 1.9769$. Therefore, the final expression for the fermionic wave-function renormalization at finite temperature and frequency (real) reads as

$$Z_\Psi\left(\frac{\omega}{T}\right) = 1 - \frac{g^2}{2}\, N_b \left[\frac{1}{\epsilon} + b + f_1\left(\frac{\omega}{T}\right)\right] \equiv 1 - \frac{g^2}{2}\, N_b \left[\frac{1}{\epsilon} + C\left(\frac{\omega}{T}\right)\right], \quad (9)$$

where $C(x) = b + f_1(x)$, yielding Eq. (11) of main text. The scaling of the function $C(x)$ with its argument is shown in Fig. 2(a) of the main paper. Notice that $Z_\Psi(x)$ is a completely real function of its argument and therefore only produces correction to the inter-band part of the OC inside the quantum critical regime of GNY QCP.

From the above expression of the fermionic self-energy correction we can arrive at the expression for the inter-band component of the OC at the GNY QCP as follows

$$\sigma^{\rm IB}_*(x) = \left(Z^2_\Psi\right)_{g^2=g^2_*} \sigma^{\rm IB}_0(x) = \left(1 - g^2_*\left[\frac{1}{\epsilon} + C\left(\frac{\omega}{T}\right)\right]\right) \sigma^{\rm IB}_0(x) = \left[1 - \frac{N_b}{2N_f}\, \left[1 + \epsilon\, C\,(x)\right]\right] \sigma^{\rm IB}_0\,(x)\,, \quad (10)$$

in agreement with Eq. (12) of main text. In the final expression for $\sigma^{\rm IB}_*(x)$ we substituted the fixed point value of the Yukawa coupling $g^2_*$, shown in Eq. (7) of the main text.

The above expression for the OC at the GNY QCP is strictly valid when the ordered phase (for $m^2_b < 0$) is an insulator or a superfluid. On the other hand, if the ordered phase represents a superconductor then the OC receives additional contribution from gapless bosonic degrees of freedom of charge $2e$, given by

$$\sigma^{\rm Bos}_* = s\, \left(Z^2_\Phi\right)_{g^2=g^2_*} \sigma^{\rm Bos}_0 = s\, \left(1 - 2N_f g^2\right)^2_{g^2=g^2_*} \sigma^{\rm Bos}_0 = s\, \left[1 - \frac{4N_f}{2N_f+4-N_b}\right] \sigma^{\rm Bos}_0 + \mathcal{O}(\epsilon), \quad (11)$$

to the leading order in the $\epsilon$-expansion, where $\sigma^{\rm Bos}_0 = \frac{8}{\pi}\, \frac{(2e)^2}{h}$, $Z_\Phi$ is the bosonic wave-function renormalization, and $s = 1$ and 3 respective for spin-singlet and triplet superconductors. Hence, the total OC at a superconducting GNY QCP is given by (to the leading order in $\epsilon$)

$$\sigma^{\rm IB}_* = \left[1 - \frac{N_b}{2N_f+4-N_b}\right] \frac{N_f\pi}{4}\, \frac{e^2}{h} + s\, \left[1 - \frac{4N_f}{2N_f+4-N_b}\right] \frac{8}{\pi}\, \frac{(2e)^2}{h} + \mathcal{O}(\epsilon). \quad (12)$$

Computation of the correction $\mathcal{O}(\epsilon)$ at such a QCP is left as a subject for a future investigation.

## II. FERMIONIC MASS AT FINITE TEMPERATURE

We now compute the thermal mass of the fermionic excitations in the quantum critical fan starting from the ordered side where both bosonic and fermionic excitations are massive. Even though both fermionic ($m_f$) and bosonic ($m_b$) masses vanish as we approach the GNY QCP from the ordered phase, their ratio tends to a universal number, which is a function of the number of bosonic ($N_b$) and fermionic ($N_f$) flavors, given by

$$\left(\frac{m_b}{m_f}\right)^2 = \frac{\lambda_*}{3g^2_*} = \frac{1}{a_3}\left[a_2 + \sqrt{a^2_2 + 16 N_f a_3}\right], \quad (13)$$

where $a_1 = 2N_f + 4 - N_b$, $a_2 = 4 - 2N_f - N_b$ and $a_3 = N_b + 8$.

Next we compute the thermal fermionic mass $[m_f(T)]$ inside the critical regime in which the physics at finite temperature is controlled by the $T=0$ GNY QCP, where both bosonic and fermionic masses satisfy $m_b(T)/T \sim m_f(T)/T \sim \sqrt{\epsilon}$, and $\lambda T/m_{b,f} \sim g^2 T/m_{b,f} \sim \sqrt{\epsilon}$, since at the quantum critical point $g_*^2 \sim \lambda_* \sim \epsilon$. To extract the thermal fermionic mass we need to compute fermionic self-energy for zero-external momentum and an external fermionic Matsubara frequency $\Omega_0$. The expression contributing to the thermal reads as

$$\Sigma_M(\Omega_0,0) = N_b g^2 T\, M_\alpha \sum_{\omega_n} \int \frac{d^d\mathbf{q}}{(2\pi)^d} \frac{m_f}{\left[\omega_n^2+q^2+m_f^2\right]\left[(\omega_n-\Omega_0)^2+q^2+m_b^2\right]} = N_b g^2 m_f \frac{S_d}{2(2\pi)^d} M_\alpha \; (\Sigma_1+\Sigma_2)\,. \tag{14}$$

We note that in the last expression $\omega_n=(2n+1)\pi T$ is the fermionic Matsubara frequency. Here, $M_\alpha$ is a $8\times 8$ *mass* matrix that fully anti-commute with the Dirac Hamiltonian.

Two parts of $\Sigma(\Omega_0,0)$ read as

$$\Sigma_1 = \int_0^\infty dq\, q^{d-1} \frac{\left(-m_b^2+m_f^2+\Omega_0^2\right)\coth\left[\frac{\sqrt{q^2+m_b^2}}{2T}\right]}{\sqrt{q^2+m_b^2}\,\left[\left(m_b^2-m_f^2\right)^2+2\left(2q^2+m_b^2+m_f^2\right)\Omega_0^2+\Omega_0^4\right]}, \tag{15}$$

$$\Sigma_2 = \int_0^\infty dq\, q^{d-1} \frac{\left(m_b^2-m_f^2+\Omega_0^2\right)\tanh\left[\frac{\sqrt{q^2+m_f^2}}{2T}\right]}{\sqrt{q^2+m_f^2}\,\left[\left(m_b^2-m_f^2\right)^2+2\left(2q^2+m_b^2+m_f^2\right)\Omega_0^2+\Omega_0^4\right]}. \tag{16}$$

To find the fermionic mass, we formally let $\Omega_0\to 0$; in other words, we impose that the fermionic mass is related to the self-energy at zero external momentum, $m_f(T)M_\alpha = -M_\alpha \Sigma_M(\Omega_0\to 0,0)$. This condition significantly simplifies the above expressions to

$$\Sigma_1 = -\frac{1}{m_b^2-m_f^2}\int_0^\infty dq\, \frac{q^{d-1}}{\sqrt{q^2+m_b^2}} \coth\left[\frac{\sqrt{q^2+m_b^2}}{2T}\right],\; \Sigma_2 = \frac{1}{m_b^2-m_f^2}\int_0^\infty dq\, \frac{q^{d-1}}{\sqrt{q^2+m_b^2}} \tanh\left[\frac{\sqrt{q^2+m_b^2}}{2T}\right]. \tag{17}$$

Now we separate the $T=0$ part from the above two expressions, since both fermionic and bosonic masses at zero temperature are zero, $m_f(0)=m_b(0)=0$. Then above two expressions further simplify to

$$\Sigma_1 = -\frac{2}{m_b^2-m_f^2}\int_0^\infty dq\, \frac{q^{d-1}}{\sqrt{q^2+m_b^2}} \frac{1}{\exp\left[\frac{\sqrt{q^2+m_b^2}}{T}\right]-1},\; \Sigma_2 = -\frac{2}{m_b^2-m_f^2}\int_0^\infty dq\, \frac{q^{d-1}}{\sqrt{q^2+m_b^2}} \frac{1}{\exp\left[\frac{\sqrt{q^2+m_b^2}}{T}\right]+1}. \tag{18}$$

To the leading order the fermionic and bosonic masses residing inside the above two integrals can be replaced by their zero temperature values, which are zero. Finally we set $d=3$. The above two expressions then finally simplify to

$$\Sigma_1 = -\frac{2}{m_b^2-m_f^2}\int_0^\infty dq\, \frac{q}{\exp[\frac{q}{T}]-1} = -\frac{2T^2}{m_b^2-m_f^2}\,\frac{\pi^2}{6},\; \Sigma_2 = -\frac{2}{m_b^2-m_f^2}\int_0^\infty dq\, \frac{q}{\exp[\frac{q}{T}]+1} = -\frac{2T^2}{m_b^2-m_f^2}\,\frac{\pi^2}{12}. \tag{19}$$

Therefore, the final expression for the thermal fermion mass reads as

$$m_f(T)M_\alpha = -M_\alpha\Sigma_M(\Omega_0\to 0,0) = \frac{N_b g^2}{m_f(T)}\, \frac{\pi^2 T^2}{\left[\left(\frac{m_b}{m_f}\right)^2-1\right]}\, M_\alpha, \tag{20}$$

yielding

$$\left(\frac{m_f(T)}{T}\right)^2 = N_b \frac{\pi^2 g^2}{\left(\frac{m_b}{m_f}\right)^2-1} = N_b \frac{\pi^2 g^2}{\frac{\lambda_*}{3g_*^2}-1} = \frac{\pi^2}{6}\,\frac{N_b}{N_f}\epsilon + \mathcal{O}\left(\frac{1}{N_f^2}\right). \tag{21}$$

While arriving at the final expression we have retained the leading order term in $1/N_f$, and rescaled $g^2/(8\pi^2)\to g^2$. Hence, finally we obtain

$$\frac{m_f(T)}{T} = \pi\sqrt{\epsilon}\,\sqrt{\frac{N_b}{6N_f}}. \tag{22}$$

## III. DERIVATION OF DRUDE CONDUCTIVITY FOR DIRAC FERMIONS

In this section we present the derivation of Drude conductivity for Dirac fermions. The polarization tensor for two-dimensional massive Dirac fermions at (bosonic) Matsubara frequency $\Omega$ and temperature $T$ is given by

$$\Pi_{lm}(i\Omega) = T\sum_{i\omega_n}\int \frac{d^2\mathbf{k}}{(2\pi)^2}\mathrm{Tr}\left[\gamma_l G_f(i\omega_n+i\Omega,\mathbf{k})\gamma_m G_f(i\omega_n,\mathbf{k})\right], \tag{23}$$

where $\omega_n$ is the fermionic Matsubara frequency, $\mathbf{k}$ is the momentum, $l,m=1,2$. The propagator of the non-interacting massive Dirac fermions reads as

$$G_f(i\omega_n,\mathbf{k}) = \frac{i\gamma_0\omega_n + i\gamma_j k_j + m_f}{\omega_n^2+E_k^2}, \tag{24}$$

where $E_k^2 = k^2+m_f^2$ and $\gamma_\mu$ ($\mu=0,j$) are the standard $\gamma-$matrices satisfying the anti-commuting Clifford algebra $\{\gamma_\mu,\gamma_\nu\}=2\delta_{\mu\nu}$. After taking the trace over the $\gamma-$matrices in Eq. (23), we obtain

$$\Pi_{lm}(i\Omega) = 4N_f\, T\sum_{i\omega_n}\int \frac{d^2\mathbf{k}}{(2\pi)^2}\frac{[\omega_n(\omega_n+\Omega)+E_k^2]\delta_{lm} - 2k_l k_m}{(\omega_n^2+E_k^2)((\omega_n+\Omega)^2+E_k^2)}. \tag{25}$$

We now set $l=m=x$ and use that $\omega_n(\omega_n+\Omega) = (\omega_n+\Omega)^2 - \Omega(\omega_n+\Omega)$, to write

$$\Pi_{xx}(i\Omega) = 4N_f\sum_{\alpha=1}^{3}\Pi_{xx}^{(\alpha)}(i\Omega), \tag{26}$$

where

$$\Pi_{xx}^{(1)}(i\Omega) = T\sum_{i\omega_n}\int\frac{d^2\mathbf{k}}{(2\pi)^2}\frac{1}{\omega_n^2+E_k^2} = T\sum_{i\omega_n}\int\frac{d^2\mathbf{k}}{(2\pi)^2}\frac{2k_x^2}{(\omega_n^2+E_k^2)^2}, \tag{27}$$

$$\Pi_{xx}^{(2)}(i\Omega) = T\sum_{i\omega_n}\int\frac{d^2\mathbf{k}}{(2\pi)^2}\frac{-2k_x^2}{(\omega_n^2+E_k^2)((\omega_n+\Omega)^2+E_k^2)}, \tag{28}$$

$$\Pi_{xx}^{(3)}(i\Omega) = T\sum_{i\omega_n}\int\frac{d^2\mathbf{k}}{(2\pi)^2}\frac{-\Omega(\omega_n+\Omega)}{(\omega_n^2+E_k^2)((\omega_n+\Omega)^2+E_k^2)}. \tag{29}$$

We performed a partial integration by inserting $1\equiv\partial k_x/\partial k_x$ and dropped the boundary piece to arrive at the final form of $\Pi_{xx}^{(1)}(i\Omega)$ in Eq. (27). The Matsubara summation appearing in this equation can compactly be written as

$$T\sum_{i\omega_n}\frac{1}{(\omega_n^2+E_k^2)^2} = \frac{1}{2E_k^2}\left\{\frac{\partial n_f(E_k)}{\partial E_k} + \frac{1}{2E_k}\left[1-2n_f(E_k)\right]\right\}, \tag{30}$$

leading to

$$\Pi_{xx}^{(1)} = \int\frac{d^2\mathbf{k}}{(2\pi)^2}\frac{k_x^2}{E_k^2}\left\{\frac{\partial n_f(E_k)}{\partial E_k} + \frac{1}{2E_k}\left[1-2n_f(E_k)\right]\right\} \equiv \Pi_{xx}^{(11)} + \Pi_{xx}^{(12)}. \tag{31}$$

Here, $n_f(z) = [e^{z/k_BT}+1]^{-1}$ is the Fermi-Dirac distribution function. The Drude component arises from the term $\Pi_{xx}^{(11)}$ in the above equation containing the derivative of the Fermi-Dirac distribution function. The term $\Pi_{xx}^{(12)}$ cancels out with the frequency independent part in the sum of the two terms $\Pi_{xx}^{(2)}$ and $\Pi_{xx}^{(3)}$. This sum ultimately yields the interband piece of the non-interacting OC, as used in the main text. The Drude part of the polarization then reads

$$\Pi_{xx}^{(D)} = 4N_f\int\frac{d^2\mathbf{k}}{(2\pi)^2}\frac{k_x^2}{E_k^2}\left(\frac{\partial n_f(E_k)}{\partial E_k}\right), \tag{32}$$

which after using Eq. (10) of the main text leads to Eq. (13) of the main text.
